# Supplementary material for: AHA!: Facilitating AI Impact Assessment by Generating Examples of Harms
Source: arXiv:2306.03280 source file (2023-06-05)
Supplement: Supplementary file 1 [file additional_analyses.tex]

\begin{table}[]
\scriptsize
\begin{tabular}{@{}lp{1.4cm}lllll}
\toprule
\rowcolor[HTML]{EFEFEF} 
Scenario    
& \begin{tabular}[c]{@{}l@{}}Crowd mean \\ (standard error)\end{tabular} 
& \begin{tabular}[c]{@{}l@{}}GPT-3 mean \\ (standard error)\end{tabular} 
& \begin{tabular}[c]{@{}l@{}}Crowd + GPT-3 \\ (standard  error)\end{tabular} 
& \begin{tabular}[c]{@{}l@{}}Crowd vs. GPT-3\end{tabular}                                     
& \begin{tabular}[c]{@{}l@{}}Crowd vs. \\ Combined\end{tabular}                               
& \begin{tabular}[c]{@{}l@{}}GPT-3 vs. \\ Combined\end{tabular}                               
\\ \midrule

\textbf{\begin{tabular}[c]{@{}l@{}}Comm. compl.\end{tabular}} & \begin{tabular}[c]{@{}l@{}}13.67 (0.83)\end{tabular}                     & \begin{tabular}[c]{@{}l@{}}14.08 (0.68)\end{tabular}                     & 19.17                                                                                             & {\color[HTML]{9B9B9B} \begin{tabular}[c]{@{}l@{}}t(22) = -0.38 p = .70 (n.s.)\end{tabular}} & {\color[HTML]{9A0000} \begin{tabular}[c]{@{}l@{}}t(22) = -4.42 p = .0002\end{tabular}}    & {\color[HTML]{9A0000} \begin{tabular}[c]{@{}l@{}}t(22) = -4.42 p = .0002\end{tabular}}    \\

\textbf{Content moder.}                                                 & \begin{tabular}[c]{@{}l@{}}13.92 (0.72)\end{tabular}                     & \begin{tabular}[c]{@{}l@{}}12.92 (0.92)\end{tabular}                     & 18.46                                                                                             & {\color[HTML]{9B9B9B} \begin{tabular}[c]{@{}l@{}}t(24) = 0.85 p = .40 (n.s.)\end{tabular}}  & {\color[HTML]{9A0000} \begin{tabular}[c]{@{}l@{}}t(24) = -3.73 p = .001\end{tabular}}     & {\color[HTML]{9A0000} \begin{tabular}[c]{@{}l@{}}t(24) = -4.13 p = .0004\end{tabular}}    \\

\textbf{Disease diag.}                                                  & \begin{tabular}[c]{@{}l@{}}8.23 (0.40)\end{tabular}                      & \begin{tabular}[c]{@{}l@{}}7.65 (0.42)\end{tabular}                      & 11                                                                                                & {\color[HTML]{9B9B9B} \begin{tabular}[c]{@{}l@{}}t(32) = 1.02 p = .32 (n.s.)\end{tabular}}  & {\color[HTML]{9A0000} \begin{tabular}[c]{@{}l@{}}t(32) = -4.58 p = 6.68e-05\end{tabular}} & {\color[HTML]{9A0000} \begin{tabular}[c]{@{}l@{}}t(32) = -5.42 p = 5.76e-06\end{tabular}} \\

\textbf{Hiring}                                                             & \begin{tabular}[c]{@{}l@{}}11.09 (0.46)\end{tabular}                     & \begin{tabular}[c]{@{}l@{}}10.91 (0.64)\end{tabular}                     & 13.58                                                                                             & {\color[HTML]{9B9B9B} \begin{tabular}[c]{@{}l@{}}t(21) = 0.23 p = .81 (n.s.)\end{tabular}}  & {\color[HTML]{9A0000} \begin{tabular}[c]{@{}l@{}}t(21) = -3.27 p = .003\end{tabular}}     & {\color[HTML]{9A0000} \begin{tabular}[c]{@{}l@{}}t(21) = -3.06 p = .006\end{tabular}}     \\

\textbf{Loan applic.}                                                   & \begin{tabular}[c]{@{}l@{}}9 (0.38)\end{tabular}                         & \begin{tabular}[c]{@{}l@{}}10.27 (0.56)\end{tabular}                     & 13.72                                                                                             & {\color[HTML]{9B9B9B} \begin{tabular}[c]{@{}l@{}}t(20) = -1.88 p = .08 (n.s.)\end{tabular}} & {\color[HTML]{9A0000} \begin{tabular}[c]{@{}l@{}}t(20) = -7.46 p = 3.38e-07\end{tabular}} & {\color[HTML]{9A0000} \begin{tabular}[c]{@{}l@{}}t(20) = -4.59 p = .0001\end{tabular}}    \\ \bottomrule
\end{tabular}
\caption{Paired t-test for means of numbers of unique codes generated by Crowd only, GPT-3 only, and Combined (Crowd + GPT-3). For all the scenarios, Crowd and GPT-3 combined generate significantly more unique codes together than either alone.}
\vspace{-8pt}
\label{table:complementarity}
\end{table}

\subsubsection{What are the distributions of harms across different generation sources and problematic outcomes?}

Disaggregating the generations further to examine the differences between sources of generation for different problematic outcomes, we again do not notice substantial differences between GPT-3 and crowds. Figure ~\ref{fig:distribution-fp-source-scenarios} shows the distribution of harms disaggregated by type of AI mistake and source of generation.

\begin{figure}[t]

\includegraphics[width=\linewidth]{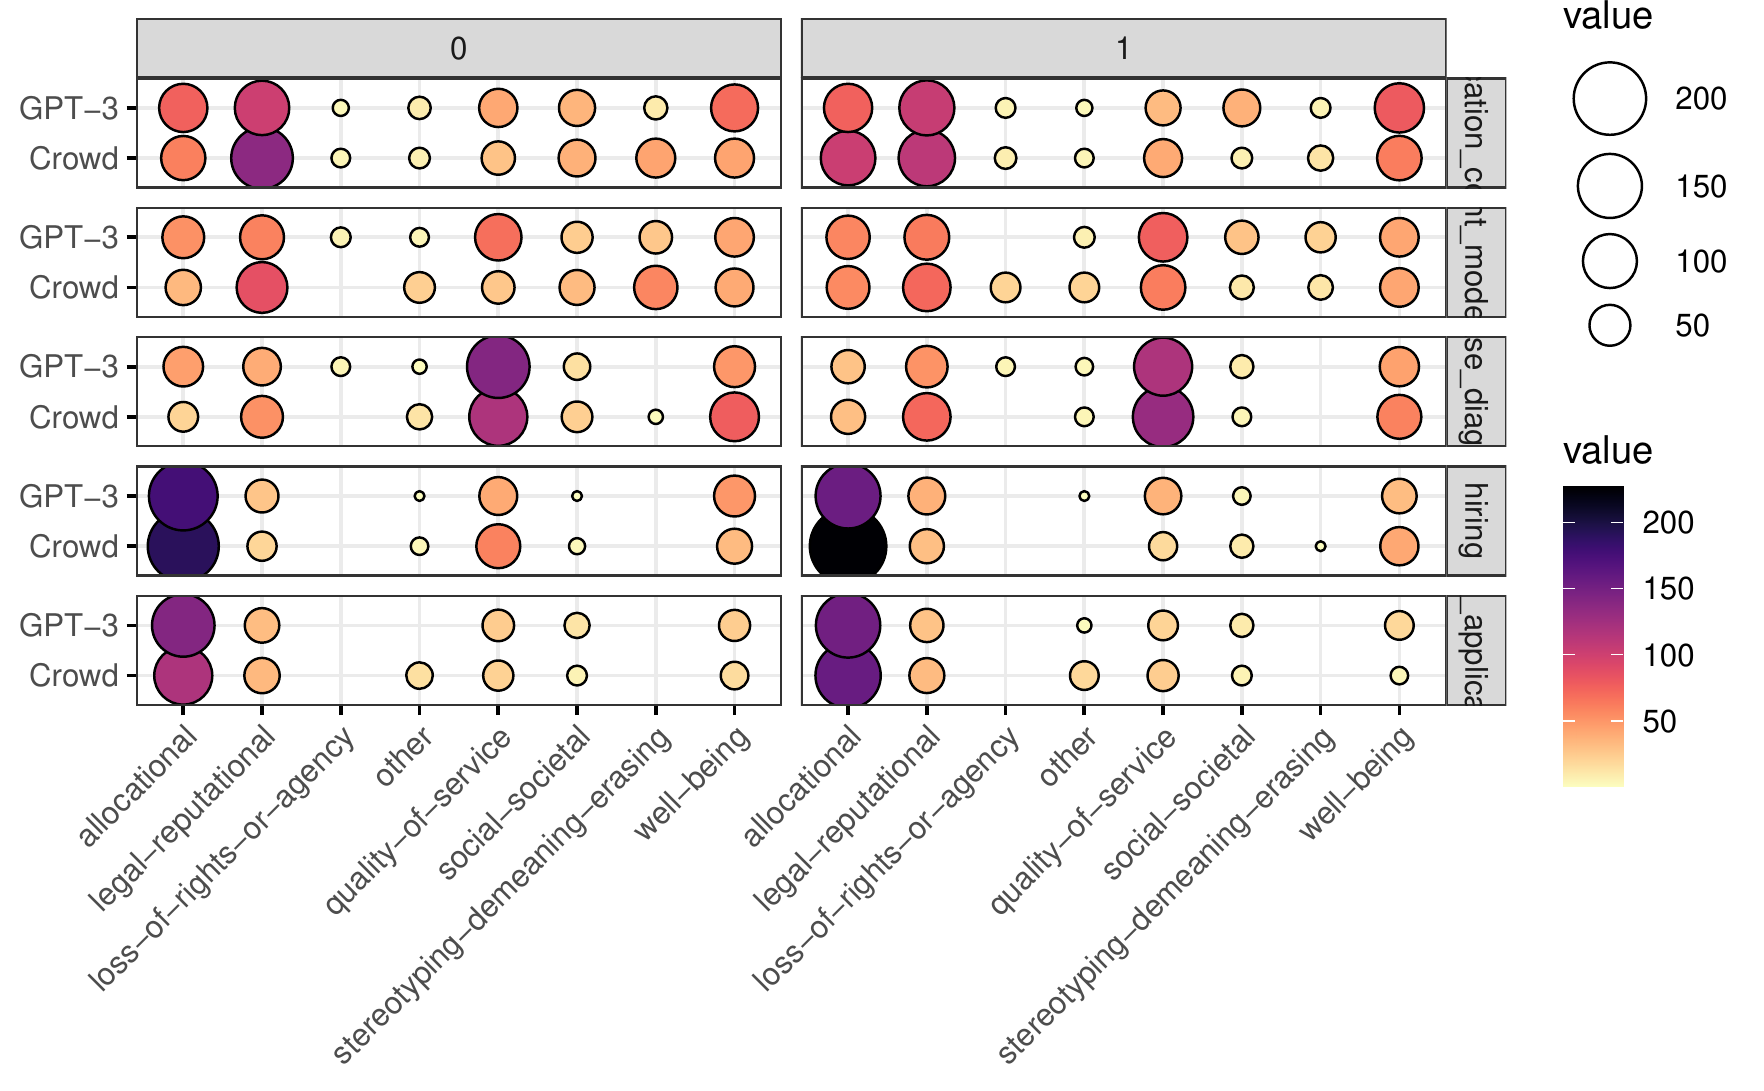}
\caption{Distribution of harms disaggregated by the type of generation source -- GPT-3 and Crowd and type of problematic outcome.} \label{fig:distribution-fp-source-scenarios}
\end{figure}

\begin{table*}[]
\begin{tabular}{lllll}
\hline
                                                                                                                          & \textbf{\begin{tabular}[c]{@{}l@{}}False \\ Positive \\ (Crowd vs. GPT-3)\end{tabular}} & \textbf{\begin{tabular}[c]{@{}l@{}}False\\ Negative\\ (Crowd vs. GPT-3)\end{tabular}} & \textbf{\begin{tabular}[c]{@{}l@{}}Crowd\\ \\ (FP vs. FN)\end{tabular}}             & \textbf{\begin{tabular}[c]{@{}l@{}}GPT-3\\ \\ (FP vs. FN)\end{tabular}}                                    \\ \hline
\rowcolor[HTML]{EFEFEF} 
\multicolumn{1}{l|}{\cellcolor[HTML]{EFEFEF}\textbf{\begin{tabular}[c]{@{}l@{}}Communication \\ compliance\end{tabular}}} & \begin{tabular}[c]{@{}l@{}}$\chi^2$(7, N=697)\\ = 530.93\\ $p < .0001$\end{tabular}     & \begin{tabular}[c]{@{}l@{}}$\chi^2$(7, N=714)\\ = 438.58\\ $p < .0001$\end{tabular}   & \begin{tabular}[c]{@{}l@{}}$\chi^2$(7, N=715)\\ = 517.15\\ $p < .0001$\end{tabular} & {\color[HTML]{333333} \begin{tabular}[c]{@{}l@{}}$\chi^2$(7, N=696)\\ = 457.29\\ $p < .0001$\end{tabular}} \\
\multicolumn{1}{l|}{\textbf{\begin{tabular}[c]{@{}l@{}}Content \\ moderation\end{tabular}}}                               & \begin{tabular}[c]{@{}l@{}}$\chi^2$(7, N=598)\\ = 233.97\\ $p < .0001$\end{tabular}     & \begin{tabular}[c]{@{}l@{}}$\chi^2$(7, N=589)\\ = 177.74\\ $p < .0001$\end{tabular}   & \begin{tabular}[c]{@{}l@{}}$\chi^2$(7, N=601)\\ = 165.34\\ $p < .0001$\end{tabular} & {\color[HTML]{333333} \begin{tabular}[c]{@{}l@{}}$\chi^2$(7, N=586)\\ = 254.3\\ $p < .0001$\end{tabular}}  \\
\rowcolor[HTML]{EFEFEF} 
\multicolumn{1}{l|}{\cellcolor[HTML]{EFEFEF}\textbf{\begin{tabular}[c]{@{}l@{}}Disease\\ diagnosis\end{tabular}}}         & \begin{tabular}[c]{@{}l@{}}$\chi^2$(6, N=569)\\ = 233.97\\ $p < .0001$\end{tabular}     & \begin{tabular}[c]{@{}l@{}}$\chi^2$(7, N=609)\\ = 695.97\\ $p < .0001$\end{tabular}   & \begin{tabular}[c]{@{}l@{}}$\chi^2$(6, N=614)\\ = 540.16\\ $p < .0001$\end{tabular} & {\color[HTML]{333333} \begin{tabular}[c]{@{}l@{}}$\chi^2$(6, N=564)\\ = 577.79\\ $p < .0001$\end{tabular}} \\
\multicolumn{1}{l|}{\textbf{Hiring}}                                                                                      & \begin{tabular}[c]{@{}l@{}}$\chi^2$(6, N=596)\\ = 1276\\ $p < .0001$\end{tabular}       & \begin{tabular}[c]{@{}l@{}}$\chi^2$(5, N=609)\\ = 916.7\\ $p < .0001$\end{tabular}    & \begin{tabular}[c]{@{}l@{}}$\chi^2$(6, N=640)\\ = 1429.6\\ $p < .0001$\end{tabular} & {\color[HTML]{333333} \begin{tabular}[c]{@{}l@{}}$\chi^2$(6, N=565)\\ = 788.1\\ $p < .0001$\end{tabular}}  \\
\rowcolor[HTML]{EFEFEF} 
\multicolumn{1}{l|}{\cellcolor[HTML]{EFEFEF}\textbf{\begin{tabular}[c]{@{}l@{}}Loan\\ application\end{tabular}}}          & \begin{tabular}[c]{@{}l@{}}$\chi^2$(5, N=476)\\ = 816.97\\ $p < .0001$\end{tabular}     & \begin{tabular}[c]{@{}l@{}}$\chi^2$(5, N=449)\\ = 579.33\\ $p < .0001$\end{tabular}   & \begin{tabular}[c]{@{}l@{}}$\chi^2$(5, N=456)\\ = 656.13\\ $p < .0001$\end{tabular} & {\color[HTML]{333333} \begin{tabular}[c]{@{}l@{}}$\chi^2$(5, N=469)\\ = 741.94\\ $p < .0001$\end{tabular}} \\ \hline
\end{tabular}
\caption{Distribution of harms disaggregated by the type of generation source -- GPT-3 and Crowd and type of problematic outcome. $\chi^2$ tests of the distributions of the types of harms for pairwise comparisons: Crowd vs. GPT-3 by type of problematic outcome (first two columns), and False Positive vs. False Negative by type of source (last two columns).}
\end{table*}

\begin{figure}[h]

\includegraphics[width=\linewidth]{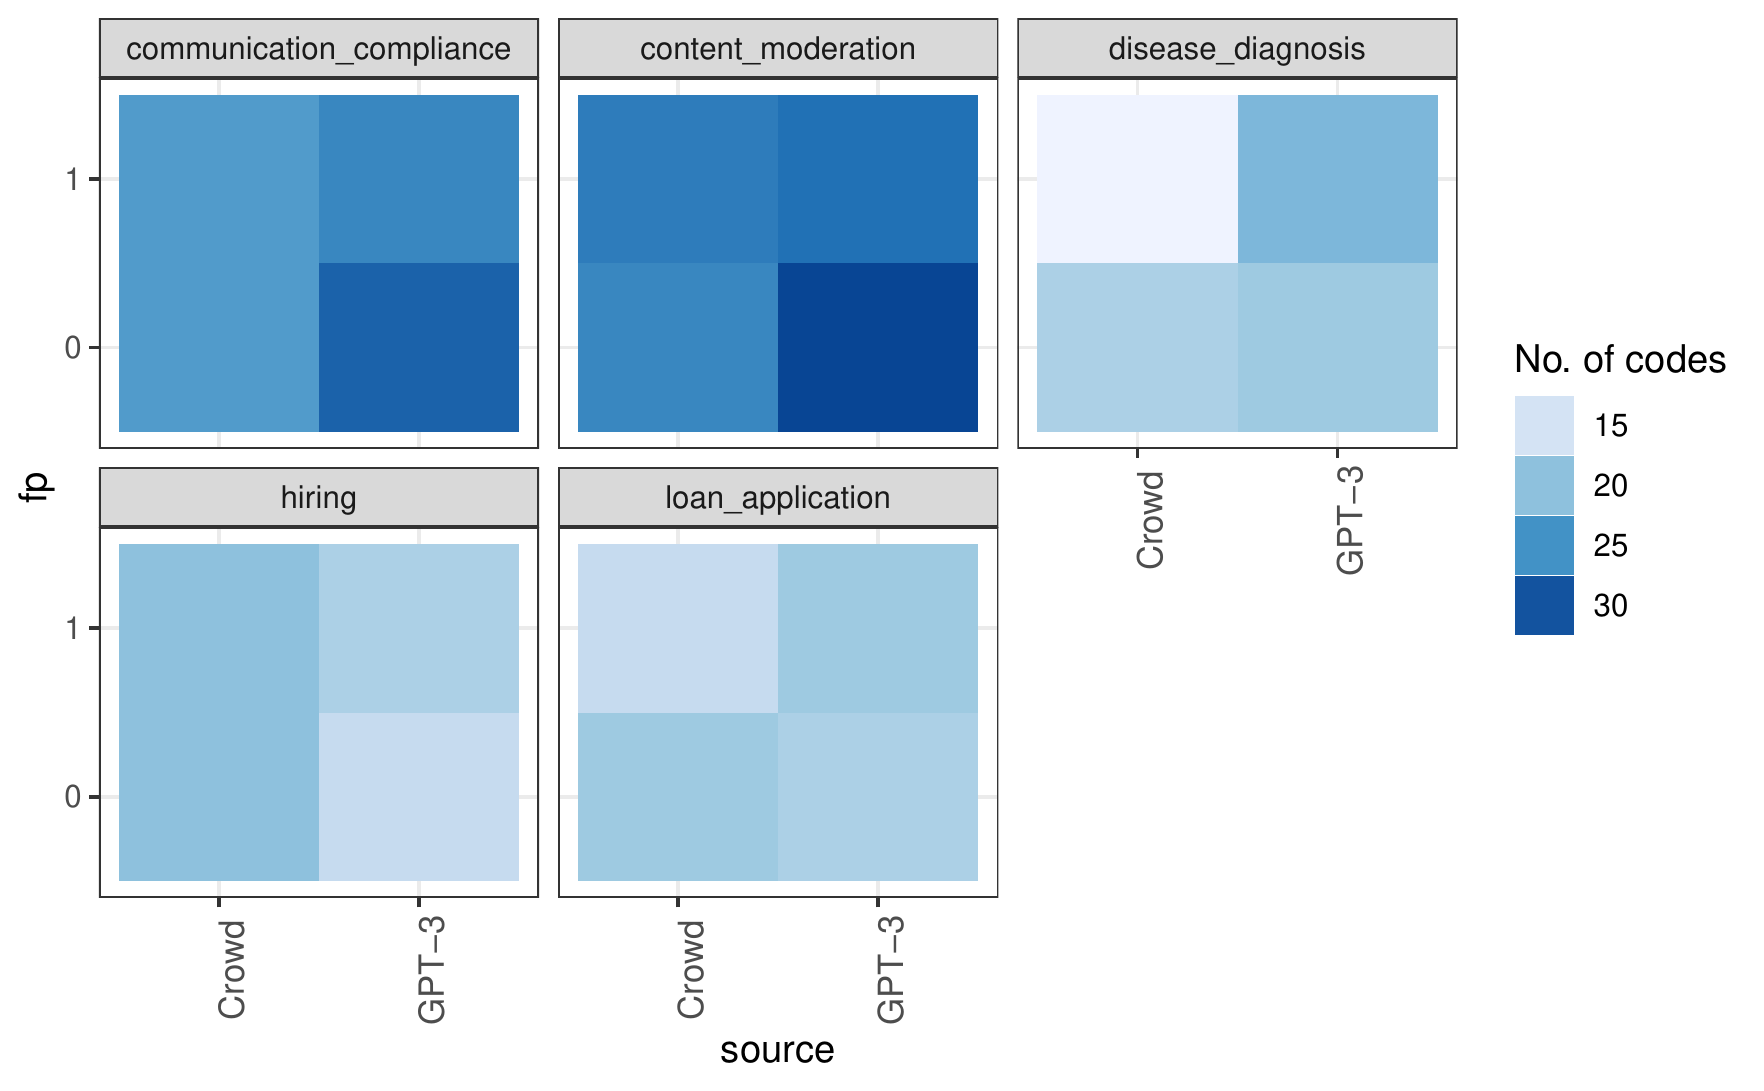}
\caption{Diversity of types of harms as measured by the number of unique codes generated by Crowd and GPT-3 for different scenarios and problematic outcomes.} \label{fig:diversity-fp-source-scenarios}
\end{figure}

\begin{figure*}
\centering
\begin{subfigure}[b]{.45\linewidth}
\includegraphics[width=\linewidth]{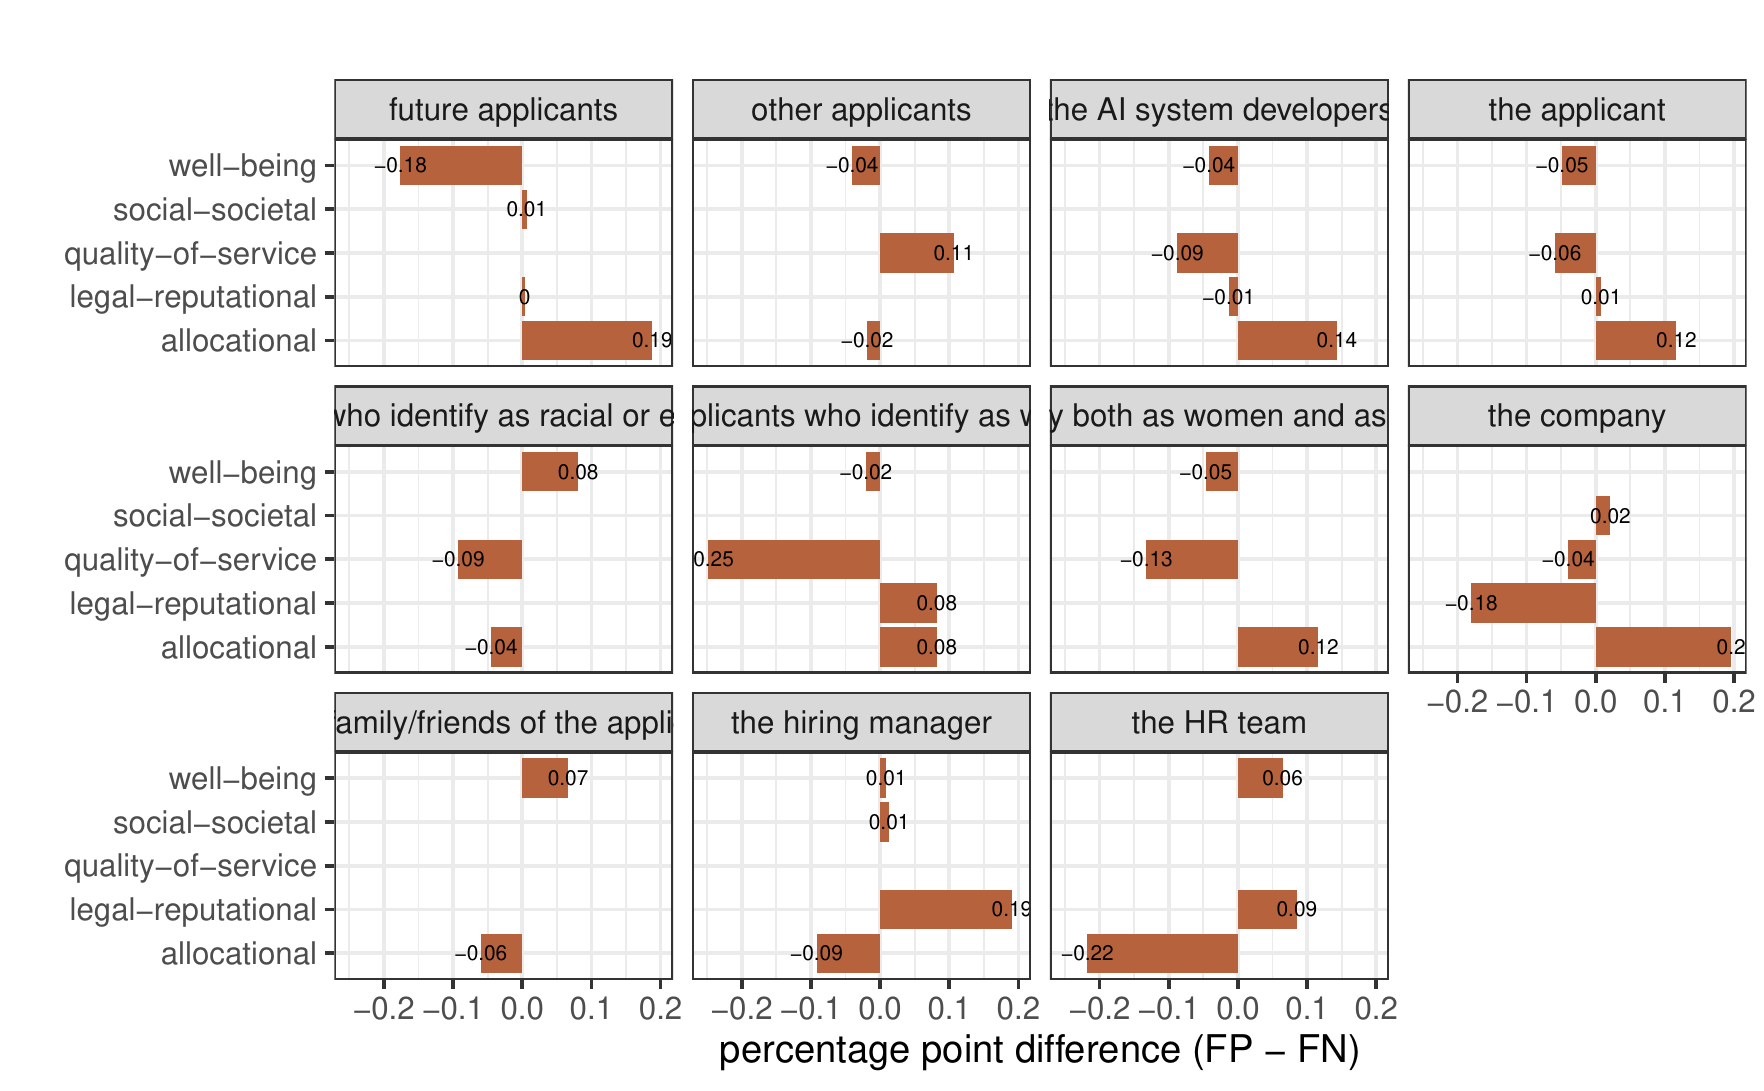}
\caption{False positive vs. false negative} 
\label{fig:distribution-fp-scenarios}
\end{subfigure}
\begin{subfigure}[b]{.45\linewidth}
\includegraphics[width=\linewidth]{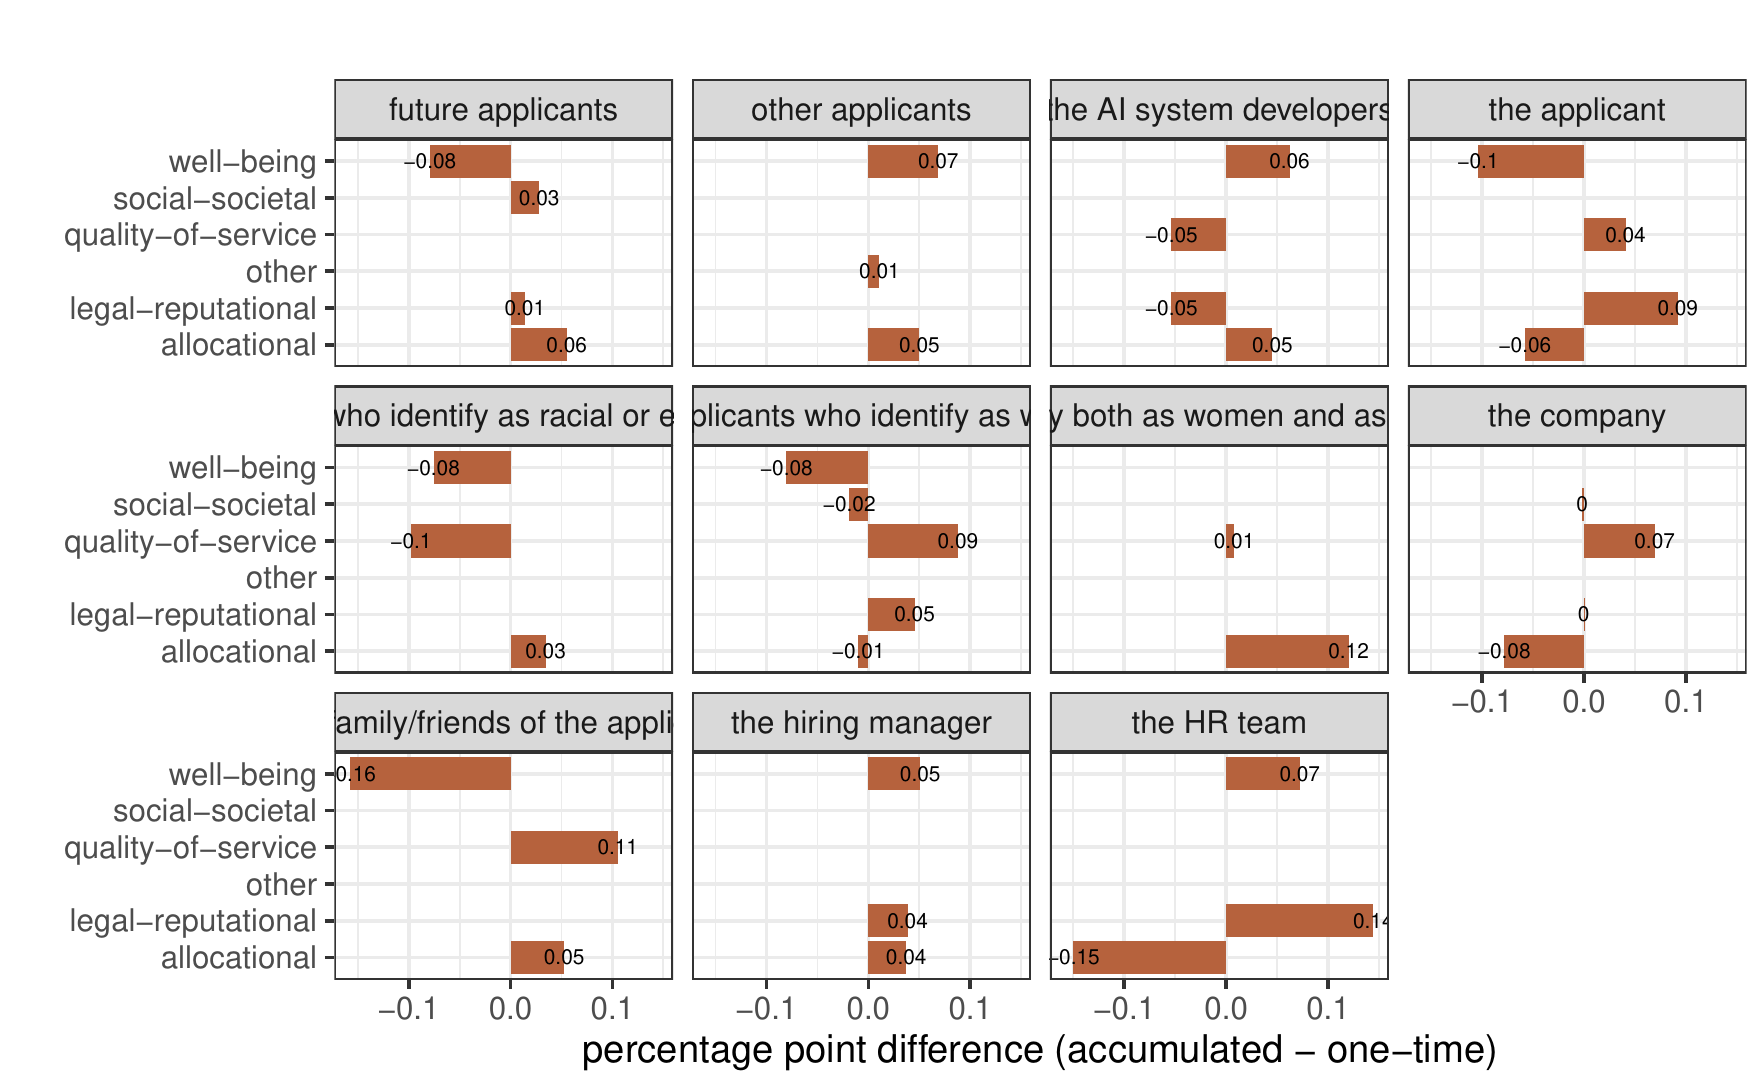}
\caption{Accumulated vs. one-time}\label{fig:accumulated_scenarios}
\end{subfigure}
\begin{subfigure}[b]{.45\linewidth}
\includegraphics[width=\linewidth]{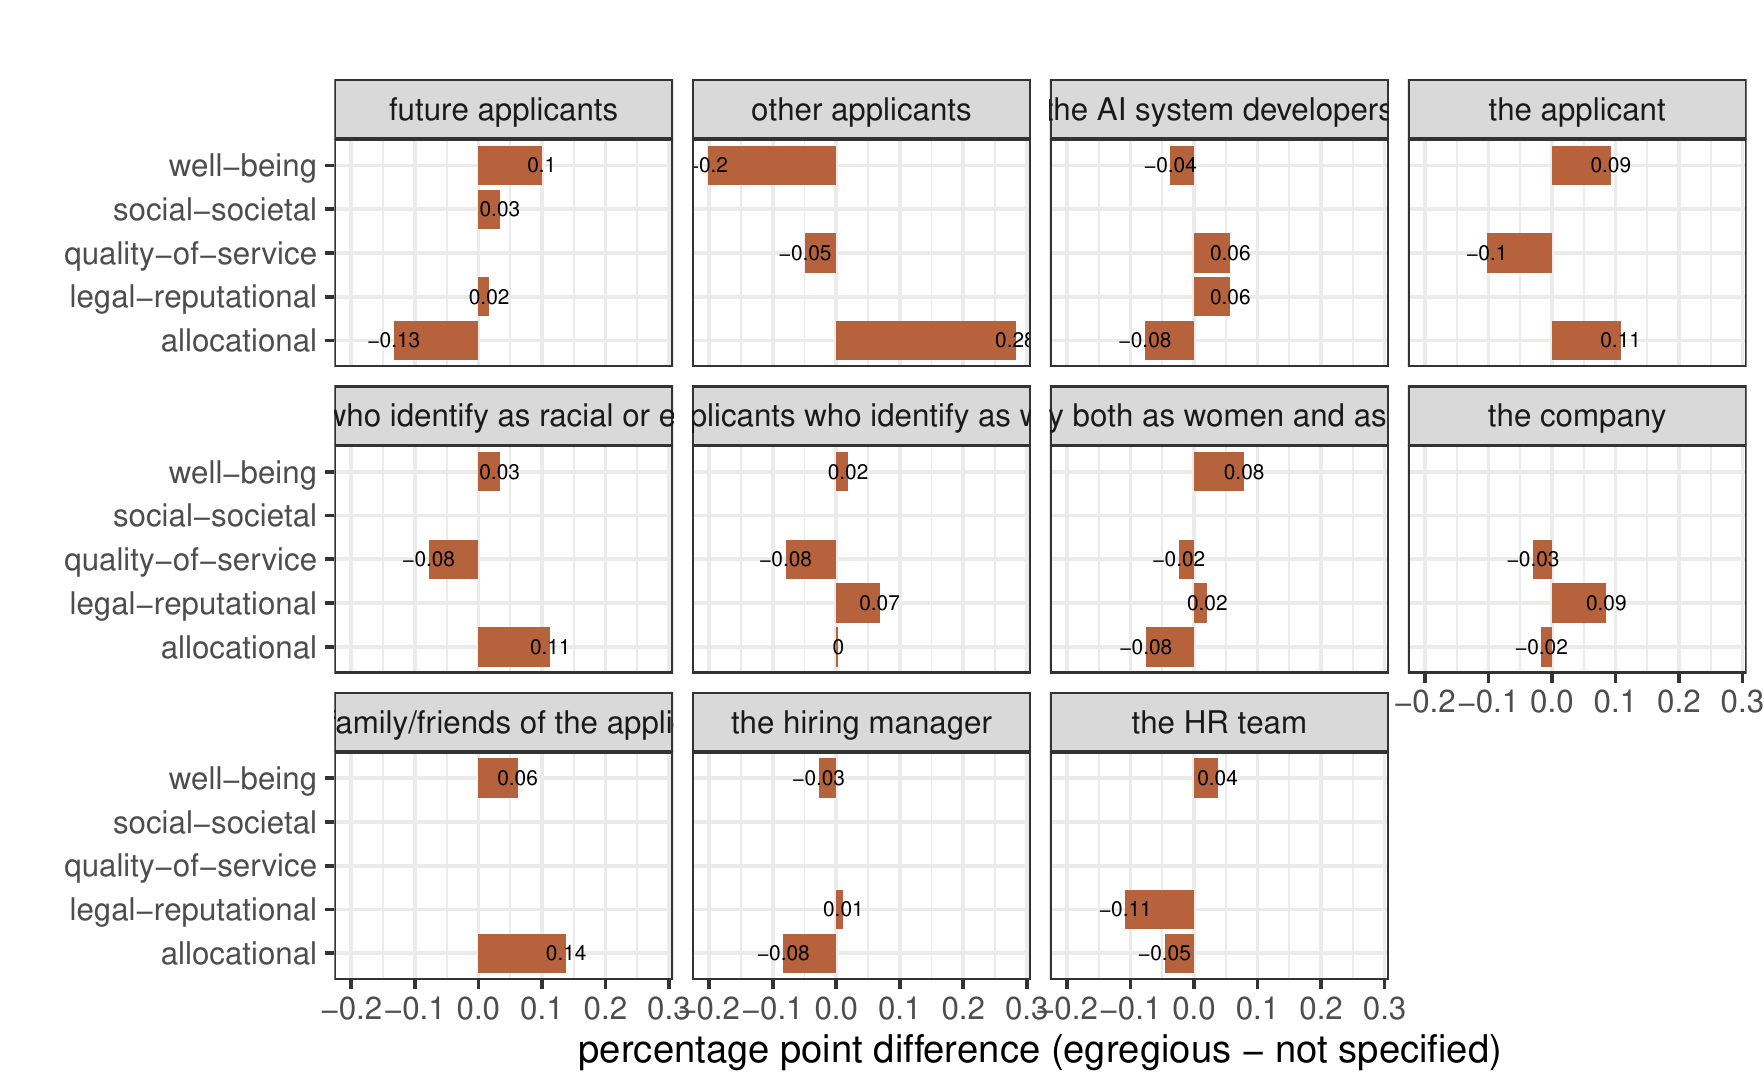}
\caption{Egregious vs. not specified}\label{fig:egregious}
\end{subfigure}
\caption{Difference in the percentage of points of the number of harms generated for different problematic outcome dimensions across stakeholders for the \em hiring \em scenario. }
\label{fig:problematic_outcomes}
\end{figure*}
